# Supplementary material for: Allocating Opportunities in a Dynamic Model of Intergenerational Mobility
Source: arXiv:2101.08451 source file (2021-01-21)
Supplement: Supplementary file 4 [file appendix_archive.tex]

\section{MDPs with Continuous State and Action Spaces}\label{app:continuous}
Finding the optimal policy for a continuous state- and action-space MDP is often a difficult task~\citep{marecki2006fast}.
Two main categories of algorithms have
been proposed to (approximately) calculate the optimal policy: 
(1) A typical approach is to \textbf{discretize} the state and action space, then solve the resulting MDP using standard methods, such policy or value iteration. This approach suffers from the well-known ``curse of dimensionality''.
(2) Another approach \textbf{approximates} the optimal value function with a parametric form, then sets out to fit those parameters such that they satisfy the Bellman equation (see, e.g., ~\citep{li2005lazy,hauskrecht2004linear}.



\section{Omitted Technical Material}

\subsection{Properties of the Value Function}\label{app:value}
In this section, we show that the value function $V(.)$ for the decision process $\cD$ is unique, continuous, differentiable, and monotonically decreasing, and concave. We begin by offering an alternative formulation of the decision process that has the exact same value function and policy, but is more conducive to recursive analysis. Next, we prove several properties of the state space $\Phi$, the action space $\Theta$, and the reward function $R$ for this alternative decision process. Then we apply previously-established theorems from dynamic programming and recursive analysis~\citep{stokey1989recursive} to establish the aforementioned properties of $V(.)$.

\paragraph{A Decision Process Equivalent to $\cD$}
Given the decision process $\cD =(\Phi, \Theta, S, R)$ (as defined in Section~\ref{sec:DP}), we first offer an alternative formulation of it, called $\cD"$, that maintains the value function and optimal policy of the original decision problem $\cD$. We construct $\cD"$ in two steps. We first construct an intermediate formulation, $\cD'$, by expanding the admissible action space of $\cD$ and the reward function. Second, we construct $\cD"$ from $\cD'$ by re-defining the action space of not in terms of thresholds, but in terms of the states reachable through an admissible threshold from every state. We also re-cast the reward function in terms of the current and the next state. The latter representation, $\cD"$ is standard in the Dynamic programming literature, and allows us to import tools and theorems with minor modification.

First, given $\cD$, we define $\cD' =(\Phi, \Theta', S, R)$ as follows: The state space $\Phi_0$ and state transition $S(.,.)$ unchanged, but we expand the set of feasible actions, $\Theta$ and the reward function $R$ as follows:
\begin{itemize}
\item $\Theta'(\phi_0) = \left[\max\left(0, \sigma \left( 1 - \frac{\alpha}{\phi_0} \right) \right), \sigma \right]$. That is, we remove the upper bound constraints on the thresholds available in each state $\phi_0 \geq 1 - \alpha$.
\item We extend the reward function as follows:
$$R'(\phi_0, \theta_0) = 
\begin{cases}
R(\phi_0, \theta_0) \quad \text{ if } \theta_0 \leq \frac{\sigma(1-\alpha)}{\phi_0}\\
\frac{\phi_0}{2\sigma} (\sigma^2 - \theta_0^2) + (1-\phi_0)\frac{\sigma+2\tau}{2} \quad \text{ if } \theta_0 > \frac{\sigma(1-\alpha)}{\phi_0}\\
\end{cases}
$$
\end{itemize}

Second, given $\cD'$, we define $\cD" =(\Phi, \Gamma, I, R")$ as follows: instead of specifying the admissible thresholds in each state, we re-define the decision process $\cD'$ in terms of the states reachable by an admissible threshold from every state. We re-cast the reward function in terms of the current and the next state, accordingly. More precisely:
\begin{itemize}
\item The correspondence $\Gamma: \Phi \rightarrow \Phi$ specifies the states reachable by one admissible $\theta_0$ from any given state $\phi_0 \in \Phi$. More precisely
$$\Gamma(\phi_0)=\{\omega \in \Phi \vert \exists \theta_0 \in \Theta'(\phi_0) \text{ s.t. }\omega = S(\phi_0, \theta_0)\}.$$
\item $I: \Phi_0 \times \Phi_0 \rightarrow \Phi_0$ simply returns its second argument, that is, for all $\phi_0 \in [0,1]$, $I(\phi_0,\omega) = \omega$.
\item To redefine the reward function in terms of the current and the next state $(\phi_0,\omega)$, note that we can write $\theta_0$ as a function of $\phi_0, \omega$ as follows:
\begin{eqnarray*}
&& \omega = \phi_0 - \frac{\phi_0}{2\sigma}(\sigma^2 - \theta^2_0) \\
&\Leftrightarrow & 2\sigma \frac{\omega}{\phi_0} + \sigma^2 - 2\sigma = \theta^2_0\\
&\Leftrightarrow & \theta_0 = \sqrt{2\sigma\frac{\omega}{\phi_0} + \sigma^2 - 2\sigma}
\end{eqnarray*}
So we can write
$$R"(\phi_0, \omega_0) = 
\begin{cases}
R' \left(\phi_0, \sqrt{2\sigma\frac{\omega}{\phi_0} + \sigma^2 - 2\sigma} \right) \quad \text{ if } \phi_0 > 0\\
R(0,0) \quad \text{ if } \phi_0 = 0
\end{cases}
$$

\end{itemize}


\begin{property}\label{4.3}
$\Phi$ is a convex subset of $\reals$, and the correspondence $\Gamma$ is nonempty, compact-valued, and continuous.
\end{property}
\begin{proof}
$\Phi = [0,1]$, which is clearly a convex subset of $\reals$. The correspondence $\Gamma$ can be characterized as follows:
%\begin{eqnarray*}
%\Gamma(\phi_0) &=&\{\phi' \in \Phi \vert \exists \theta_0 \in \Theta(\phi_0) \text{ s.t. }\phi' = S(\phi_0, \theta_0)\} \\
%&=& \left\{ \phi' \in \Phi \vert \phi' = \phi_0 - \frac{\phi_0}{2\sigma} (\sigma^2 - \theta_0^2) \text{ where } \sigma \left( 1 - \frac{\alpha}{\phi_0} \right) \leq \theta_0 \leq \frac{\sigma(1-\alpha)}{\phi_0} \text{ and } 0 \leq \theta_0 \leq 1 \right\} \\
%&=& \begin{cases}
%               \phi_0' \in \left[\phi_0\left(1-\frac{1}{2\sigma}\right) , \phi_0\right] \quad \text{ if } \phi_0 \leq \alpha\\
%               \phi_0' \in \left[\phi_0-\sigma\alpha \left(1+\frac{\alpha}{2\phi_0}\right) , \phi_0\right] \quad \text{ if } \alpha < \phi_0 \leq 1-\alpha\\
%               \phi_0' \in \left[\phi_0-\sigma\alpha \left(1+\frac{\alpha}{2\phi_0}\right)  , \phi_0-\frac{\phi_0}{2\sigma} \left( 1 - \frac{1-\alpha}{\phi_0} \right)\left( 1 + \frac{1-\alpha}{\phi_0} \right)\right] \quad \text{ if } \phi_0 \geq 1-\alpha
%            \end{cases}
%            \\
%&=& \left[ \max \left\{ \phi_0\left(1-\frac{1}{2\sigma}\right), \phi_0-\sigma\alpha \left(1+\frac{\alpha}{2\phi_0}\right) \right\}  , \min\left\{ \phi_0, \phi_0-\frac{\phi_0}{2\sigma} \left( 1 - \frac{1-\alpha}{\phi_0} \right)\left( 1 + \frac{1-\alpha}{\phi_0} \right) \right\}\right]            
%\end{eqnarray*}
\begin{eqnarray*}
\Gamma(\phi_0) &=&\{\omega \in \Phi \vert \exists \theta_0 \in \Theta'(\phi_0) \text{ s.t. }\omega = S(\phi_0, \theta_0)\} \\
&=& \left\{ \omega \in \Phi \vert \omega = \phi_0 - \frac{\phi_0}{2\sigma} (\sigma^2 - \theta_0^2) \text{ where } \sigma \left( 1 - \frac{\alpha}{\phi_0} \right) \leq \theta_0 \leq \sigma \text{ and }  \theta_0 \geq 0 \right\} \\
&=& \begin{cases}
               \omega \in \left[\phi_0\left(1-\frac{1}{2\sigma}\right) , \phi_0\right] \quad \text{ if } \phi_0 \leq \alpha\\
               \omega \in \left[\phi_0-\sigma\alpha \left(1-\frac{\alpha}{2\phi_0}\right) , \phi_0\right] \quad \text{ if } \phi_0 \geq \alpha\\
            \end{cases}
            \\
&=& \left[ \max \left\{ \phi_0\left(1-\frac{1}{2\sigma}\right), \phi_0-\sigma\alpha \left(1-\frac{\alpha}{2\phi_0}\right) \right\} , \phi_0 \right]            
\end{eqnarray*}
which is clearly nonempty, compact-valued, and continuous.
\end{proof}

\begin{property}\label{4.8}
$\Gamma$ is convex.
\end{property}
\begin{proof}
Recall that 
$$\Gamma(\phi_0) = \left[ \max \left\{ \phi_0\left(1-\frac{1}{2\sigma}\right), \phi_0-\sigma\alpha \left(1-\frac{\alpha}{2\phi_0}\right) \right\}  , \phi_0 \right].$$
Note that the upper-bound $\phi_0$ is a concave function of $\phi_0$. 
Furthermore, the lower bound is a convex function of $\phi_0$, because:
\begin{itemize}
\item $\phi_0\left(1-\frac{1}{2\sigma}\right)$ is a linear (and therefore convex) function of $\phi_0$.
\item $\phi_0-\sigma\alpha \left(1-\frac{\alpha}{2\phi_0}\right)$ is a convex function of $\phi_0$.
\item The pointwise maximum of two convex functions is convex.
\end{itemize}
Therefore, $\Gamma(\phi_0)$ is the area between the intersection of a concave upper-boundary and a convex lower-boundary, hence, it is convex.
\end{proof}

\begin{property}\label{4.4}
The reward function $R"$ is bounded and continuous.
\end{property}
\begin{proof}
The reward function $R$ specifies the fraction of the population who succeed if given the opportunity. So clearly $0 \leq R(.,.) \leq 1$ is bounded. As a result $R"$ is also bounded.

To establish continuity of $R"$, we first establish the continuity of $R'$. Recall that
$$R'(\phi_0, \theta_0) = 
\begin{cases}
R(\phi_0, \theta_0) \quad \text{ if } \theta_0 \leq \frac{\sigma(1-\alpha)}{\phi_0}\\
\frac{\phi_0}{2\sigma} (\sigma^2 - \theta_0^2) + (1-\phi_0)\frac{\sigma+\tau}{2} \quad \text{ if } \theta_0 > \frac{\sigma(1-\alpha)}{\phi_0}\\
\end{cases}
$$

\textbf{Case 1 $\left( \theta_0 \leq \frac{\sigma(1-\alpha)}{\phi_0}\right)$:}
It is trivial to see that $R(.,.)$ (defined in (\ref{eq:reward})) is continuous at any $\phi_0<1$. At $\phi_0 = 1$, we have
\begin{eqnarray*}
&& \lim_{\phi_0 \rightarrow 1} \frac{\phi_0}{2\sigma} (\sigma^2 - \theta_0^2)
+ \frac{1-\phi_0}{2\sigma} \left((\sigma+\tau)^2 - \left( \frac{\sigma(1-\alpha) + (1-\phi_0)\tau - \phi_0 \theta_0}{1-\phi_0}\right)^2\right)\\
&=& \frac{1}{2\sigma} (\sigma^2 - \theta_0^2) - \lim_{\phi_0 \rightarrow 1} 
\frac{1-\phi_0}{2\sigma} \left( \frac{\sigma(1-\alpha) + (1-\phi_0)\tau - \phi_0 \theta_0}{1-\phi_0}\right)^2\\
&=& \frac{1}{2\sigma} (\sigma^2 - \theta_0^2) - \lim_{\phi_0 \rightarrow 1} 
\frac{1}{2\sigma}  \frac{\left(\sigma(1-\alpha) + (1-\phi_0)\tau - \phi_0 \theta_0\right)^2}{1-\phi_0}\\
&=& \frac{1}{2\sigma} (\sigma^2 - \theta_0^2) - \lim_{\phi_0 \rightarrow 1} 
\frac{1}{2\sigma}  \frac{\left(\sigma(1-\alpha) + (1-\phi_0)\tau - \phi_0 \sigma(1-\alpha)\right)^2}{1-\phi_0}\\
\text{(L'Hospital's rule)}&=& \frac{1}{2\sigma} (\sigma^2 - \theta_0^2) - \lim_{\phi_0 \rightarrow 1} 
\frac{1}{\sigma}  \frac{ (\tau+\sigma(1-\alpha))\left(\sigma(1-\alpha) + (1-\phi_0)\tau - \phi_0 \sigma(1-\alpha)\right)}{1}\\
&=& \frac{1}{2\sigma} (\sigma^2 - \theta_0^2) - 0\\
 &=& \frac{1}{2\sigma} (\sigma^2 - \theta_0^2) \\
 &=& R(\theta_0, 1).
\end{eqnarray*}
So $R$ is continuous at $\phi_0 = 1$, as well.

\vspace{3mm}
\textbf{Case 2 $\left( \theta_0 > \frac{\sigma(1-\alpha)}{\phi_0}\right)$:} Note that $R'(\phi_0, \theta_0) = \frac{\phi_0}{2\sigma} (\sigma^2 - \theta_0^2) + (1-\phi_0)\frac{\sigma+2\tau}{2}$, which is obviously continuous.

To establish the continuity of $R'$, it only remains to show that for all $\phi_0$, $R'(\phi_0, .)$ is continuous at $\theta'_0 = \frac{\sigma(1-\alpha)}{\phi_0}$. That is,
$$\lim_{\theta_0 \rightarrow \theta'_0} R(\phi_0, \theta_0) = \lim_{\theta_0 \rightarrow \theta'_0} \frac{\phi_0}{2\sigma} (\sigma^2 - \theta_0^2) + (1-\phi_0)\frac{\sigma+\tau}{2}$$
To prove this, we can write:
\begin{eqnarray*}
\lim_{\theta_0 \rightarrow \theta'_0} R(\phi_0, \theta_0) &=& \lim_{\theta_0 \rightarrow \theta'_0} \frac{\phi_0}{2\sigma} (\sigma^2 - \theta_0^2)
+ \frac{1-\phi_0}{2\sigma} \left((\sigma+\tau)^2 - \left( \frac{\sigma(1-\alpha) + (1-\phi_0)\tau - \phi_0 \theta_0}{1-\phi_0}\right)^2\right)\\
&=& \frac{\phi_0}{2\sigma} (\sigma^2 - {\theta'_0}^2)
+ \frac{1-\phi_0}{2\sigma} \left((\sigma+\tau)^2 - \left( \frac{\sigma(1-\alpha) + (1-\phi_0)\tau - \phi_0 \theta'_0}{1-\phi_0}\right)^2\right)\\
&=& \frac{\phi_0}{2\sigma} (\sigma^2 - {\theta'_0}^2)
+ \frac{1-\phi_0}{2\sigma} \left((\sigma+\tau)^2 - \left( \frac{\sigma(1-\alpha) + (1-\phi_0)\tau - \phi_0 \frac{\sigma(1-\alpha)}{\phi_0}}{1-\phi_0}\right)^2\right)\\
&=& \frac{\phi_0}{2\sigma} (\sigma^2 - {\theta'_0}^2)
+ \frac{1-\phi_0}{2\sigma} \left((\sigma+\tau)^2 -\tau^2\right)\\
&=& \frac{\phi_0}{2\sigma} (\sigma^2 - {\theta'_0}^2)
+ \frac{1-\phi_0}{2} \left(\sigma+2\tau\right)\\
&=& \lim_{\theta_0 \rightarrow \theta'_0} \frac{\phi_0}{2\sigma} (\sigma^2 - {\theta'_0}^2) + (1-\phi_0)\frac{\sigma+2\tau}{2}
\end{eqnarray*}

Finally, note that $\sqrt{2\sigma\frac{\omega}{\phi_0} + \sigma^2 - 2\sigma}$ is continuous function of $\phi_0, \omega$, so $R"$ is also continuous. \hh{More detail TBD.}
\end{proof}


Let $C(\Phi)$ be the space of bounded continuous functions $f:\Phi_0 \rightarrow \reals$ with the sup norm $\Vert f \Vert = \max_{\phi_0 \in \Phi} \vert f(\phi_0)\vert$.
We define the operator $T$ on the space $C(\Phi)$ as follows:
$$(Tf)(\phi_0) = \max_{\omega \in \Gamma(\phi_0)} R"(\phi_0,\omega) + \gamma f(\omega).$$

\begin{theorem}[Adapted version of Theorem 4.6 in \citep{stokey1989recursive}] Let $\Phi$, $\Gamma$, and $R"$ satisfy Properties~\ref{4.3} and \ref{4.4}. Then the operator $T$ maps $C(\Phi)$ into itself, $T:C(\Phi) \rightarrow C(\Phi)$, and $T$ has a unique fixed point $V \in C(\Phi)$. Moreover, given $V$, the optimal policy correspondence $\Pi^*: \Phi \rightarrow \Phi$ is compact-valued and upper hemi continuous (u.h.c).
\end{theorem}

According to \citet{cotter2006non}, if the reward function $R"$ is differentiable, the value function $V$ is differentiable on any interior point that is an optimal ``next state'' for some current state. More precisely,

\begin{theorem}[Adapted version of Theorem 2 in \citep{cotter2006non}]
Suppose $\omega \in \Pi^*(\phi_0) \cap (0,1)$ for some $\phi_0 \in [0,1]$. If $R"$ is continuously differentiable, then $V$ is differentiable at $\omega$, with $V'(\omega)=R"_{\phi_0}(\omega, \omega')$ for all $\omega' \in \Pi^*(\omega)$.
\end{theorem}

It only remains to show that:
\begin{property}\label{4.9}
$R"$ is continuously differentiable on the interior of its domain.
\end{property}
\begin{proof}
First, we show that $R'$ is continuously differentiable on the interior of its domain. To establish continuous differentiablity of $R'$ in $\theta$, note that:
$$\dd{\theta_0} R'(\phi_0, \theta_0) = 
\begin{cases}
\dd{\theta_0} R(\phi_0, \theta_0) \quad \text{ if } \theta_0 \leq \frac{\sigma(1-\alpha)}{\phi_0}\\
-\frac{\phi_0 \theta_0}{\sigma} \quad \text{ if } \theta_0 > \frac{\sigma(1-\alpha)}{\phi_0}
\end{cases}
$$

\begin{eqnarray*}
\lim_{\theta_0 \rightarrow \frac{\sigma(1-\alpha)}{\phi_0}} \dd{\theta_0} R(\phi_0, \theta_0) &=&  \lim_{\theta_0 \rightarrow \frac{\sigma(1-\alpha)}{\phi_0}}  \frac{\phi_0}{\sigma} \left( \frac{\sigma(1-\alpha) + (1-\phi_0)\tau - \theta_0}{1-\phi_0} \right)\\
&=&  \frac{\phi_0}{\sigma} \left( \frac{\sigma(1-\alpha) + (1-\phi_0)\tau -  \frac{\sigma(1-\alpha)}{\phi_0}}{1-\phi_0} \right)
\end{eqnarray*}

\begin{eqnarray*}
\dd{\theta_0} R'(\phi_0, \theta_0) &=& \dd{\theta_0} R(\phi_0, \theta_0) \\
&=&  \frac{\phi_0}{\sigma} \left( \frac{\sigma(1-\alpha) + (1-\phi_0)\tau - \theta_0}{1-\phi_0} \right).
\end{eqnarray*}

Second, we observe that:
\begin{eqnarray*}
\dd{\omega} R"(\phi_0, \omega) &=& \dd{\theta_0} R'(\phi_0, \theta_0) \dd{\omega} \theta_0 \\
&=&  \dd{\theta_0} R'(\phi_0, \theta_0) \times \frac{\sigma}{\sqrt{2\sigma\omega\phi_0 + (\sigma^2 - 2\sigma)\phi_0^2}}.
\end{eqnarray*}
\end{proof}

\iffalse

\iffalse
\begin{property}\label{4.5}
For each $\theta$, $R(.,\theta)$ is strictly decreasing in its first argument.
\end{property}
\begin{proof}
Intuitively, for a fixed threshold $\theta_0$, as we increase the proportion of the disadvantaged, the immediate reward we obtain goes down. More formally,
\begin{eqnarray*}
\dd{\phi_0} R(\phi_0, \theta_0) &=& \frac{1}{2\sigma} (\sigma^2 - \theta_0^2) + \frac{-1}{2\sigma} \left((\sigma+\tau)^2 - \left( \frac{\sigma(1-\alpha) + (1-\phi_0)\tau - \phi_0 \theta_0}{1-\phi_0}\right)^2\right) \\
&&+ \frac{-1}{\sigma} \left( \frac{\sigma(1-\alpha) + (1-\phi_0)\tau - \phi_0 \theta_0}{1-\phi_0}\right) \left( \frac{-\theta_0+ \sigma(1-\alpha))}{1-\phi_0}\right)
\end{eqnarray*}
\end{proof}

\begin{property}\label{4.6}
$\Gamma$ is monotone in the sense that $\phi_0<\phi_0'$ implies $\Gamma(\phi_0')\subseteq \Gamma(\phi_0)$.
\end{property}
\begin{proof}

\end{proof}

\begin{theorem}[Adapted version of Theorem 4.7 in \citep{stokey1989recursive}] 
Let $\Phi$, $T$, and $R"$ satisfy Properties~\ref{4.3}--\ref{4.6}, and let $V$ be the unique solution to (\ref{eq:bellman}). Then $V$ is strictly increasing.
\end{theorem}
\fi

\begin{property}\label{4.7}
$R'$ is strictly concave.
\end{property}
\begin{proof}
%Forming the Hessian matrix of $R$, we have 
%$$ \mathbf {H} ={\begin{bmatrix}
%{\dfrac {\partial ^{2}R}{\partial {\phi_0^2}}} & {\dfrac {\partial ^{2}R}{\partial \phi_0\,\partial \theta_0}}
%\\[2.2ex]{\dfrac {\partial ^{2}R}{\partial {\theta_0^2}}} & {\dfrac {\partial ^{2}R}{\partial \theta_0\,\partial \phi_0}}
%\end{bmatrix}}.$$
%where 
%$$\dfrac {\partial ^{2}R}{\partial {\phi_0^2}} = \frac{1}{\sigma} \left(\frac{\sigma(1-\alpha)-\theta_0}{(1-\phi_0)^2}\right) \left(\frac{\sigma(1-\alpha) -\theta_0}{1-\phi_0}\right) <0$$
%$$\dfrac {\partial ^{2}R}{\partial \phi_0\,\partial \theta_0} = -\frac{\theta_0}{\sigma}  -\frac{\theta_1}{\sigma}\left(\phi_0 + \frac{1+\phi_0}{1-\phi_0} \right) -\frac{1}{\sigma} \left( \frac{\phi_0}{1-\phi_0} (\theta_0 + \tau)\right) < 0$$
%$$\dfrac {\partial ^{2}R}{\partial {\theta_0^2}} = \frac{-\phi_0}{\sigma(1-\phi_0)} <0$$
%$$\dfrac {\partial ^{2}R}{\partial \theta_0\,\partial \phi_0} = \frac{\sigma(1-\alpha) +(1-\phi_0)\tau - \theta_0}{(1-\phi_0)^2}>0$$
%Using the above inequalities, it is easy to see that the determinant of $H$ is negative, therefore $R$ is strictly concave.

\hh{Incomplete! I believe the property does not hold for $R'$.}
\end{proof}



\begin{theorem}[Adapted version of Theorem 4.8 in \citep{stokey1989recursive}] 
Let $\Phi$, $\Gamma$, and $R"$ satisfy Properties~\ref{4.3}, \ref{4.4}, \ref{4.7}, and \ref{4.8}; let $V$ be the optimal value function and $\Pi$ the optimal value correspondence. Then $V$ is strictly concave and $\Pi$ is a continuous, single-valued function.
\end{theorem}

Given the definition of $R'(.,.)$, it is easy to see that:
\begin{property}\label{4.9}
$R'$ is continuously differentiable on the interior of its domain.
\end{property}
%\begin{proof}
%Clear! \hh{TBA.}
%\end{proof}

\begin{theorem}[Adapted version of Theorem 4.11 in \citep{stokey1989recursive}] 
Let $\Phi$, $\Gamma$, and $R"$ satisfy Properties~\ref{4.3}, \ref{4.4}, \ref{4.7}, \ref{4.8}, and \ref{4.9}. If $\phi_0 \in \text{int } \Phi$ and $S(\phi_0, \theta^*_0) \in \text{int } \Phi$, then $V$ is continuously differentiable at $\Phi_0$.%, with derivatives given by ...
\end{theorem}
\fi

The following corollary establishes that the value function (of the optimal policy) is decreasing.
\begin{corollary}[The Slope of the Value Function]\label{cor:value}
Let $V(\phi_0)$ denote the value of state $0 \leq \phi_0 \leq 1$. $V'(\phi_0)<0$ for every $0 \leq \phi_0 \leq 1$. 
\end{corollary}
\begin{proof}
First note that for any $\phi_0 \leq \phi^*_0$, $V'(\phi_0)<0$. Utilizing (\ref{eq:partial_value}), we have
$$\dd{\phi_0} V(\phi_0) = -\frac{\sigma \alpha^2}{2(1-\gamma)(1-\phi_0)^2} <0.$$
Second, since $V(\phi_0)$ is concave, $V'(\phi_0)$ can only decrease with $\phi_0$. Therefore, for $\phi_0 > \phi^*_0$, $V'(\phi_0)<0$.
\end{proof}
%\begin{proof}
%Recall that
%\begin{equation*}
%V(\phi_0) = \max_{\theta_0} R(\phi_0, \theta_0) + \gamma V(S(\phi_0, \theta_0))
%\end{equation*}
%Let $f(\theta_0; \phi_0) \equiv R(\phi_0, \theta_0) + \gamma V(S(\phi_0, \theta_0))$. 
%Let $\theta_0^*(\phi_0)$ denote the maximizer of $f(\theta_0; \phi_0)$.
%So we have
%\begin{eqnarray*}
%\dd{\phi_0} V &=& \dd{\phi_0}\theta^*_0  \dd{\theta_0} f + \dd{\phi_0} f \\
%&=& \dd{\phi_0}\theta^*_0  \times 0 + \dd{\phi_0} f \\
%&=& \dd{\phi_0} f \\
%&=& \dd{\phi_0} R(\phi_0, \theta^*_0) + \gamma \dd{\phi_0}S(\phi_0, \theta^*_0)  \dd{\phi_0}V(S(\phi_0, \theta^*_0))\\
%&=& \dd{\phi_0} R(\phi_0, \theta^*_0) + \gamma \dd{\phi_0}S(\phi_0, \theta^*_0)  \dd{\phi_0}V(S(\phi_0, \theta^*_0))\\
%\end{eqnarray*}
%It is easy to see that
%$$\dd{\phi_0} S(\phi_0, \theta^*_0) = 1 - \frac{\sigma^2 - \theta^{*2}_0}{2\sigma} \geq 1 - \frac{\sigma^2}{2\sigma} = 1 -\sigma/2 > 0.$$
%Note that $\dd{\phi_0} R(\phi_0, \theta^*_0)$ is equal to
%\begin{eqnarray*}
%&&  \frac{1}{2\sigma} (\sigma^2 - \theta_0^2) + \frac{-1}{2\sigma} \left((\sigma+\tau)^2 - \left( \frac{\sigma(1-\alpha) + (1-\phi_0)\tau - \phi_0 \theta_0}{1-\phi_0}\right)^2\right) \\
%&&+ \frac{1-\phi_0}{2\sigma} (-2) \left( \frac{\sigma(1-\alpha) + (1-\phi_0)\tau - \phi_0 \theta_0}{1-\phi_0}\right) \left( \frac{-(\tau + \theta_0)(1-\phi_0) + \sigma(1-\alpha) + (1-\phi_0)\tau - \phi_0 \theta_0)}{(1-\phi_0)^2}\right)\\
%&=&  \frac{1}{2\sigma} (\sigma^2 - \theta_0^2) + \frac{-1}{2\sigma} \left((\sigma+\tau)^2 - \left( \frac{\sigma(1-\alpha) + (1-\phi_0)\tau - \phi_0 \theta_0}{1-\phi_0}\right)^2\right) \\
%&&+ \frac{-1}{\sigma} \left( \frac{\sigma(1-\alpha) + (1-\phi_0)\tau - \phi_0 \theta_0}{1-\phi_0}\right) \left( \frac{-\theta_0+ \sigma(1-\alpha))}{1-\phi_0}\right)
%\end{eqnarray*}
%\end{proof}

\subsection{Derivation of $\gamma^*$, $\tau^*$, and $\alpha^*$}
Note that 
\begin{eqnarray*}
1 - \frac{\alpha \sigma}{2\tau} \left( 1 + \sqrt{1 + \frac{2\tau\gamma}{1-\gamma}}\right)
& \leq &  1 - \frac{\alpha \sigma}{2\tau} \left( 1 + 1\right)\\
& \leq &  1 - \frac{\alpha \sigma}{\tau}
\end{eqnarray*}
If $\tau < \alpha \sigma$, then $1 - \frac{\alpha \sigma}{\tau} < 1- 1 = 0$ and $\phi^*_0 = 0$. So in what follows, we assume $\tau > \alpha \sigma$ .

\paragraph{Derivation of $\gamma^*$}
Assuming that $\alpha, \tau, \sigma, \gamma \in (0,1)$ and $\tau > \sigma \alpha$, 
\begin{eqnarray*}
&& 1 - \frac{\alpha \sigma}{2\tau} \left( 1 + \sqrt{1 + \frac{2\tau\gamma}{1-\gamma}}\right) \leq 0\\
&\Leftrightarrow & 1 \leq \frac{\alpha \sigma}{2\tau} \left( 1 + \sqrt{1 + \frac{2\tau\gamma}{1-\gamma}} \right)\\
&\Leftrightarrow & \frac{2\tau}{\alpha \sigma} \leq  1 + \sqrt{1 + \frac{2\tau\gamma}{1-\gamma}} \\
&\Leftrightarrow & \frac{2\tau}{\alpha \sigma} - 1\leq   \sqrt{1 + \frac{2\tau\gamma}{1-\gamma}} \\
&\Leftrightarrow & \left( \frac{2\tau}{\alpha \sigma} - 1 \right)^2 \leq   1 + \frac{2\tau\gamma}{1-\gamma} \\
&\Leftrightarrow & \left( \frac{2\tau}{\alpha \sigma} - 1 \right)^2 - 1 \leq   \frac{2\tau\gamma}{1-\gamma} \\
&\Leftrightarrow & \frac{1}{2\tau}\left( \frac{2\tau}{\alpha \sigma} - 1 \right)^2 - \frac{1}{2\tau} \leq   \frac{\gamma}{1-\gamma} \\
&\Leftrightarrow & 1 - \left( \frac{1}{2\tau}\left( \frac{2\tau}{\alpha \sigma} - 1 \right)^2 - \frac{1}{2\tau} + 1 \right)^{-1} \leq   \gamma \\
\end{eqnarray*}

\paragraph{Derivation of $\tau^*$}
Assuming that $\alpha > 0$, $\tau, \gamma \in (0,1)$, $\sigma = 1-\tau$ and $2\tau > \sigma \alpha$, 
\begin{eqnarray}
&& 1 - \frac{\alpha \sigma}{2\tau} \left( 1 + \sqrt{1 + \frac{2\tau\gamma}{1-\gamma}}\right) \leq 0 \nonumber\\
&\Leftrightarrow & 1 \leq \frac{\alpha \sigma}{2\tau} \left( 1 + \sqrt{1 + \frac{2\tau\gamma}{1-\gamma}} \right) \nonumber\\
\text{(assuming $\alpha> 0$ and $0 < \tau < 1$)} &\Leftrightarrow & \frac{2\tau}{\alpha \sigma} \leq  1 + \sqrt{1 + \frac{2\tau\gamma}{1-\gamma}}  \nonumber\\
&\Leftrightarrow & \frac{2\tau}{\alpha \sigma} - 1\leq   \sqrt{1 + \frac{2\tau\gamma}{1-\gamma}}  \nonumber\\
\text{(assuming $2\tau > \alpha (1-\tau)$)}  &\Leftrightarrow & \left( \frac{2\tau}{\alpha \sigma} - 1 \right)^2 \leq   1 + \frac{2\tau\gamma}{1-\gamma} \nonumber\\
&\Leftrightarrow & \frac{4\tau^2}{\alpha^2 \sigma^2} - \frac{4\tau}{\alpha \sigma} + 1 \leq   1 + \frac{2\tau\gamma}{1-\gamma} \nonumber\\
&\Leftrightarrow & \frac{4\tau^2}{\alpha^2 \sigma^2} - \frac{4\tau}{\alpha \sigma} \leq    \frac{2\tau\gamma}{1-\gamma}  \nonumber\\
\text{divide by $\tau$ assuming $\tau >0$)}   &\Leftrightarrow & \frac{2\tau}{\alpha^2 \sigma^2} - \frac{2}{\alpha \sigma} \leq    \frac{\gamma}{1-\gamma}  \nonumber\\
&\Leftrightarrow & 2\tau - 2\alpha \sigma \leq    \frac{\gamma \alpha^2 \sigma^2}{1-\gamma}  \nonumber\\
&\Leftrightarrow & 2\tau - 2\alpha (1-\tau) \leq    \frac{\gamma \alpha^2}{1-\gamma} (1-\tau)^2  \nonumber\\
&\Leftrightarrow & 2 - 2 + 2\tau - 2\alpha (1-\tau) \leq    \frac{\gamma \alpha^2}{1-\gamma} (1-\tau)^2  \nonumber\\
&\Leftrightarrow & 2 - 2(1-\tau) - 2\alpha (1-\tau) \leq    \frac{\gamma \alpha^2}{1-\gamma} (1-\tau)^2  \nonumber\\
&\Leftrightarrow & 0 \leq   \frac{\gamma \alpha^2}{1-\gamma} (1-\tau)^2  + 2(1+\alpha)(1-\tau) - 2 \nonumber\\
&\Leftrightarrow & 0 \leq   \frac{\gamma \alpha^2}{2(1-\gamma)} (1-\tau)^2  + (1+\alpha)(1-\tau) - 1 \nonumber\\
&\Leftrightarrow & \tau \leq   1- \frac{-(1+\alpha) + \sqrt{ (1+\alpha)^2 + \frac{2\gamma \alpha^2}{(1-\gamma)}}}{\frac{\gamma \alpha^2}{(1-\gamma)}} \label{eq:tau_star}
\end{eqnarray}
where the last line is derived by obtaining the roots of the quadratic function $q(x) = \frac{\gamma \alpha^2}{2(1-\gamma)} x^2  + (1+\alpha)x - 1$, as follows:
\begin{equation*}
x^*_{1} = \frac{-(1+\alpha) - \sqrt{ (1+\alpha)^2 + \frac{2\gamma \alpha^2}{(1-\gamma)}}}{\frac{\gamma \alpha^2}{(1-\gamma)}} \text{  ,  } x^*_{2} = \frac{-(1+\alpha) + \sqrt{ (1+\alpha)^2 + \frac{2\gamma \alpha^2}{(1-\gamma)}}}{\frac{\gamma \alpha^2}{(1-\gamma)}}.
\end{equation*}
Note that $\frac{\gamma \alpha^2}{2(1-\gamma)} > 0$, so $q(x) \geq 0$ if and only if $x < x^*_{1}$ or $x > x^*_{2}$. Note that $x^*_{1}<0$ so if we know $x$ is positive, then $q(x) \geq 0$ if and only if $x > x^*_{2}$. Replacing $x$ with $(1-\tau)$, gives us equation (\ref{eq:tau_star}).

\paragraph{Derivation of $\alpha^*$}
Assuming that $\tau \in (0,1)$ and $\gamma < 1$,
\begin{eqnarray*}
&& 1 - \frac{\alpha \sigma}{2\tau} \left( 1 + \sqrt{1 + \frac{2\tau\gamma}{1-\gamma}}\right) \leq 0\\
&\Leftrightarrow & 1 \leq \frac{\alpha \sigma}{2\tau} \left( 1 + \sqrt{1 + \frac{2\tau\gamma}{1-\gamma}} \right)\\
&\Leftrightarrow & \frac{2\tau}{\sigma} \left( 1 + \sqrt{1 + \frac{2\tau\gamma}{1-\gamma}} \right)^{-1} \leq  \alpha
\end{eqnarray*}
